# Supplementary material for: Asynchronous Credit Assignment for Multi-Agent Reinforcement Learning
Source: arXiv:2408.03692 source file (2025-05-19)
Supplement: Supplementary file 1 [file 18_appendix.tex]

\section{Performance on Original POAC Scenarios}
\label{app:original_poac}

In the original POAC benchmark, infantry, chariots, and tanks move at speeds of 0.2, 1, and 1, respectively. This means that only infantry movement requires five time steps, with all other actions concluding in one. This limited asynchronicity in the original POAC does not fully demonstrate the strengths of our asynchronous credit assignment method. Therefore, in this paper, we adjust the movement speeds of infantry, chariots, and tanks to 0.2, 0.3, and 0.5, as shown in Table \ref{tab:attribution}.

\begin{figure}[h]
	\centering
	\includegraphics[width=1\textwidth]{pic//bq_all_ori}
	\caption{Test win rate \% on all scenarios of the original POAC benchmark.}
	\label{fig:bq_all_ori}
\end{figure}

To comprehensively evaluate the performance of our proposed MVD, we also conducted experiments across five scenarios in the original POAC benchmark. The experimental results are presented in Figure \ref{fig:bq_all_ori}. We observe that our MVD maintains competitive performance. Since most decisions in the original POAC are synchronous, all VD algorithms can achieve similar performance. Especially in scenario 2, MVD and NA$^2$Q possess high representational capabilities and exhibit similar performance, while VDN, QMIX, and Qatten, which have limited representational abilities, also show comparable results. MAC IAICC can still learn slowly in complex scenarios. However, IPPO, where each agent is trained independently, fails to converge in the scenarios that demand strong cooperation. Similar to Figure \ref{fig:bq_all}, in the scenario 1, both IPPO and MAC IAICC rapidly converge to the optimal joint strategy. However, owing to the simplicity of the original POAC, other algorithms gradually converge to the same performance as well.
